# Supplementary material for: Modulation of ionic conduction using polarizable surfaces
Source: arXiv:2306.10214 source file (2023-10-11)
Supplement: Supplementary file 1 [file supplementary_material.pdf]

# Modulation of ionic conductance using polarizable surfaces: Supplemental Material


Alexandre P. dos Santos

*Instituto de Física, Universidade Federal do Rio Grande do Sul,*
*Caixa Postal 15051, CEP 91501-970, Porto Alegre, RS, Brazil. and*
*Department of Materials Science and Engineering,*
*Northwestern University, Evanston, Illinois 60208, USA*

Felipe Jiménez-Ángeles

*Department of Materials Science and Engineering,*
*Northwestern University, Evanston, Illinois 60208, USA*

Ali Ehlen

*Applied Physics Program, Northwestern University, Evanston, Illinois 60208, USA*

Monica Olvera de la Cruz

*Department of Materials Science and Engineering, Evanston, Illinois 60208, USA and*
*Department of Physics and Astronomy,*
*Northwestern University, Evanston, Illinois 60208, USA*



(Dated: October 11, 2023)

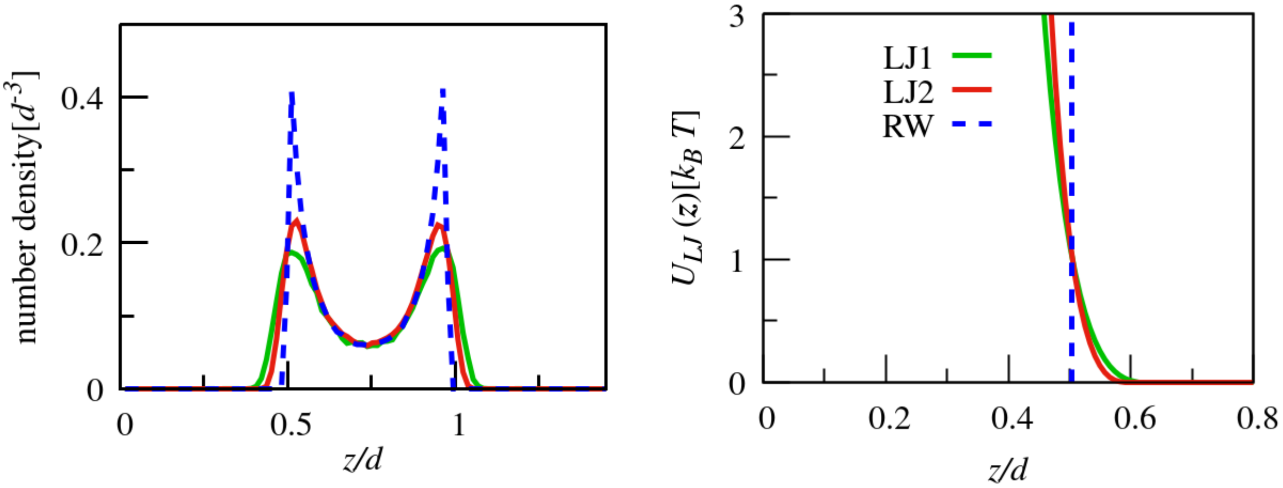


Figure S1: Effect of the softness (Lennard-Jones energy) of the conducting confining walls, for $E = 0$. (a) Number density profiles as a function of the position in the slit channel using walls of different softness and (b) the corresponding wall interaction potential $u(z)$. LJ1 refers to a Lennard-Jones wall with $\sigma_{\mathrm{LJ}} = 0.39$ nm, used in the main text, LJ2 refers to $\sigma_{\mathrm{LJ}} = 0.29$ nm, and RW represents a reflective wall, where the $z$ component of the velocity of any ion crossing the wall is instantaneously flipped. The dielectric constant in the space between the two surfaces is $\varepsilon_{\mathrm{w}} = 5\varepsilon_0$ and $l_B = 26.4d$, as in the main text. Ions absorb to the confining walls in all cases, but the softness of the walls impacts the quantitative shape of their distribution.

## Walls model

We use a truncated Lenard-Jones potential to model the interaction between the ions and the wall with an origin $z_0$ given by $U_{\mathrm{LJ}}(z) = 4\epsilon_{\mathrm{LJ}} \left[ \left( \frac{\sigma_{\mathrm{iw}}}{z-z_0} \right)^{12} - \left( \frac{\sigma_{\mathrm{iw}}}{z-z_0} \right)^{6} + 1/4 \right]$ for $z \leq z_c \equiv z_0 + 2^{1/6}\sigma_{\mathrm{iw}}$, and $U_{\mathrm{LJ}}(z) = 0$ for $z > z_c$, where $\epsilon_{\mathrm{LJ}} = k_B T$ and $\sigma_{\mathrm{iw}} = (\sigma_{\mathrm{LJ}} + d)/2$, being $\sigma_{\mathrm{LJ}}$ and $d$ the wall's and ion's Lenard-Jones diameters, respectively. We define the wall's surface as $z_s$, where $z_0 = z_s - \sigma_{\mathrm{LJ}}/2$. Fig. S1 shows the ion density profile for conductors for different wall softness, modified by the choice of $\sigma_{\mathrm{LJ}}$. We notice that the ions' distribution is sensitive to the walls' softness, but the qualitative adsorbtion behavior does not change.

For calculation of induced polarization charges in *explicit polarization* models, we place the polarizable sites at locations $\{\mathbf{R}_i\}$ on a plane at $z_0$ or $z_s$ in a two-dimensional planar mesh. In the main text, we use a hexagonal (graphene) pattern, but the mesh pattern can affect ion-surface interaction. Ionic currents resulting from changing the mesh type and size are shown in Fig. S2. Triangular meshes with smaller side lengths give ionic currents that are closer to those calculated using the Green function method. However, meshing raises the question of whether perfectly

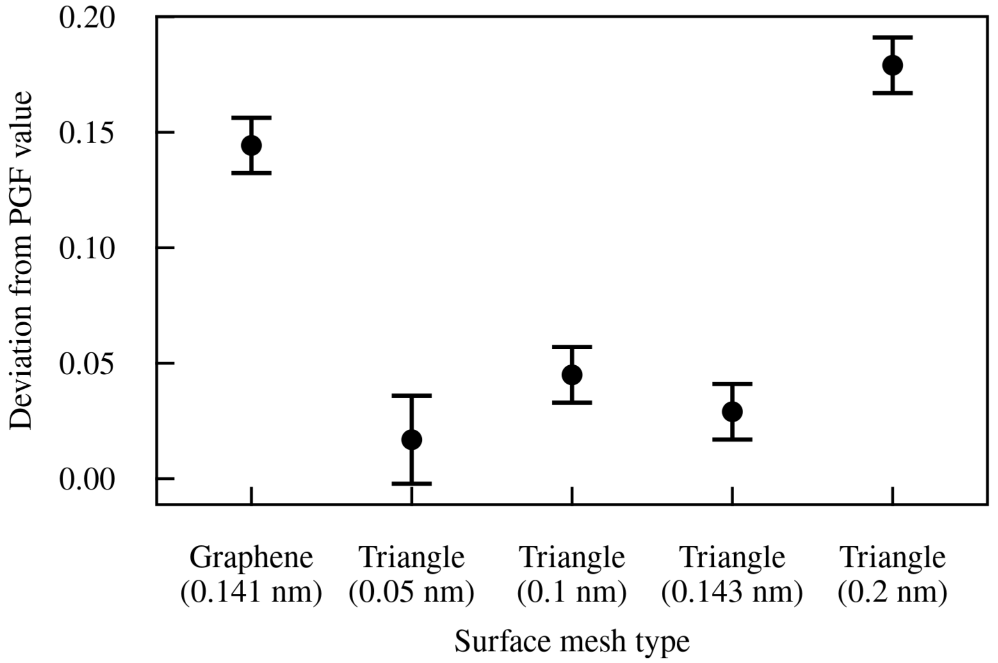


Figure S2: Analysis of the effect of surface meshing of polarization charge points for *explicit polarization* models. This figure shows the ionic current difference between the PGF and *explicit polarization* models (*surface* placement), for dielectric confinement with $E = 8.275\ \mathrm{k_BTe^{-1}d^{-1}}$, as a function of surface mesh type for a fixed box size. Current from the *explicit polarization* models ($I_{\mathrm{pol}}$) is quantified as a deviation from the PGF value ($I_{\mathrm{PGF}}$)), which is calculated as: $(I_{\mathrm{pol}} - I_{\mathrm{PGF}})/I_{\mathrm{PGF}}$. Graphene meshing is used in the main text, and thus the graphene point in this plot also appears in Fig. 4. All other points use a triangular mesh, with sizes varying as indicated. All simulations except the 0.05 nm mesh were run for 30 ns. These data indicate that placing polarization charge points on a finer mesh could improve the agreement between models in Fig. 4.
*Note:* The error bars for the 0.05 nm triangular mesh are larger than the others because this simulation is computationally expensive, and it was run for 13 ns instead of 30. We expect it to fully converge after another 7 ns.

smeared or more localized polarization charge better represents a surface in conditions of such strong confinement and small length scales. This is worth further consideration and depends on the system to be studied, as discussed in Section 5.2.2 of [1].

## Conductors Model

The electrostatic boundary conditions determine the induced polarization surface charges. In the *polarization* models, we use a grid, consisting of $N_g$ nodes located at $\{\mathbf{R}_i\}$ in a hexagonal (graphene) mesh, to place the polarization charges. For conductors, we assign the polarization

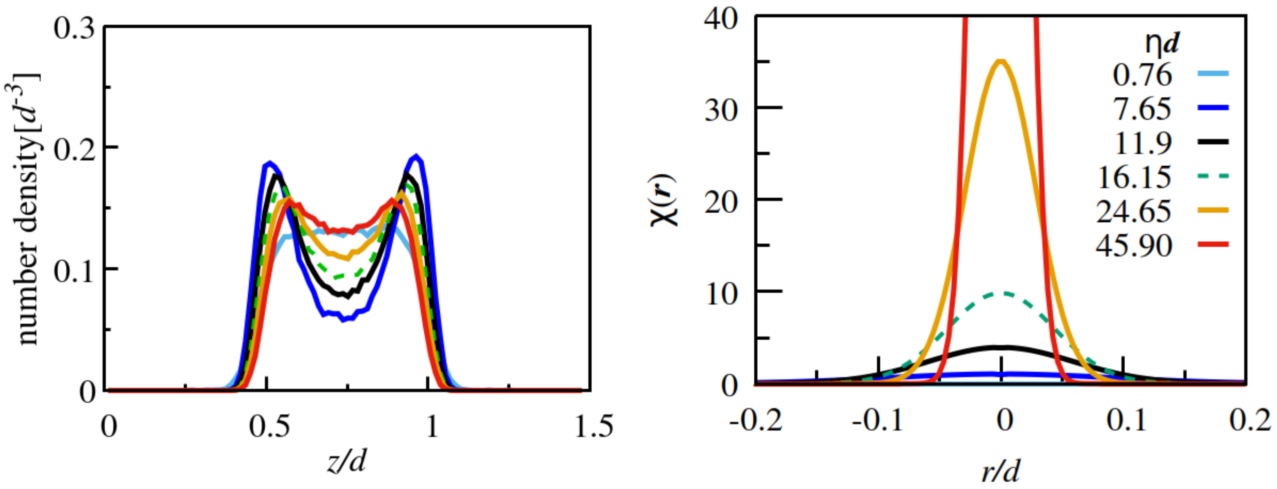


Figure S3: Effect of the polarization charge distribution width ($\eta$) in the *explicit polarization* model for conductors with *surface* charge placement, as implemented in [3]. Here we show how the ion density is modified by changing $\eta$. (a) Ion number density profiles as a function of the position in the slit channel at different values of $\eta$ and (b) the corresponding Gaussian charge distribution, $\chi(r)$. The dielectric constant in the space between the two surfaces is $\varepsilon_{\mathrm{w}} = 5\varepsilon_0$ and $l_B = 26.4d$, as in the main text.

charge at each grid point $\mathbf{R}_i$ using a Gaussian distribution [2] as $\rho_i(\mathbf{r}) = q_i\chi_i(\mathbf{r})$ where $\chi_i(\mathbf{r}) = (\frac{\eta^2}{\pi})^{3/2}\exp\{-\eta^2(\mathbf{r}-\mathbf{R}_i)^2\}$. The inverse width of the distribution $\eta$ is a measure of how tightly bound electrons are to surface nuclei, which affects short-range ion-surface interaction [1]. It is not entirely clear how to select the value of $\eta$, which may be material- and configuration-dependent, but some value of $\eta$ are unrealistic and don't appropriately model a constant potential surface. For a longer discussion of the value of $\eta$, see Chapter 5 of [1] (which uses the symbol $\eta$ for this quantity). We chose $\eta$ by comparing ion densities between the Green function method (FSCC) and the conducting *explicit polarization* method with *surface* polarization charge placement. Ion densities for varying values of $\eta$ are shown in Fig. S3. In our study, we set $\eta$=2.8 ($\eta d = 11.9$) which is the value for which the ion density agrees with the Green function method.

Note that the *explicit polarization* model for dielectric surfaces does not include a similar parameter, because surface charge is distributed as $N_g$ point charges exactly at $\{\mathbf{R}_i\}$.

[1] T. Gingrich, *Simulating Surface Charge Effects in Carbon Nanotube Templated Ionic Crystal Growth*, Ph.D. thesis, University of Oxford (2010).

[2] F. Jiménez-Ángeles, A. Ehlen, and M. Olvera de la Cruz, Faraday Discussions (2023), DOI:10.1039/D3FD00028A.

[3] L. J. V. Ahrens-Iwers, M. Janssen, S. R. Tee, and R. H. Meißner, J. Chem. Phys. **157**, 084801 (2022).
